# Supplementary material for: GAS-NeRF: Geometry-Aware Stylization of Dynamic Radiance Fields
Source: arXiv:2503.08483 source file (2025-03-11)
Supplement: Supplementary file 1 [file X_suppl.tex]

\clearpage
\setcounter{page}{1}

\maketitlesupplementary

\bigskip

\begin{minipage}[h]{0.9\textwidth}
\centering
% \FloatBarrier % This ensures tables stay in place
% \begin{table}[ht!]

% \begin{subtable}[t]{0.9\textwidth}
  \centering
  \begin{tabular}{l cc cc cc cc cc}
    \toprule
    \multirow{2}{*}{Method} & \multicolumn{2}{c}{Flame Salmon} & \multicolumn{2}{c}{Coffee Martini} & \multicolumn{2}{c}{Cook Spinach} & \multicolumn{2}{c}{Flame Steak} & \multicolumn{2}{c}{Cut Roasted Beef} \\
    \cmidrule(lr){2-3} \cmidrule(lr){4-5} \cmidrule(lr){6-7} \cmidrule(lr){8-9} \cmidrule(lr){10-11}
    & RGB$\downarrow$ & Depth$\downarrow$ & RGB$\downarrow$ & Depth$\downarrow$ & RGB$\downarrow$ & Depth$\downarrow$ & RGB$\downarrow$ & Depth$\downarrow$ & RGB$\downarrow$ & Depth$\downarrow$ \\
    \midrule
    ARF*~\cite{arf} & 6.49 & 8.42 & 6.56 & 8.77 & 6.57 & 8.85 & 6.45 & 8.89 & \underline{6.37} & 9.12 \\
    Ref-NPR*~\cite{zhang2023ref} & 6.56 & 8.42 & 6.70 & 8.77 & 6.69 & 8.85 & 6.69 & 8.89 & 6.77 & 9.12 \\
    S-DyRF~\cite{li2024sdyrf} & \textbf{6.23} & 8.42 & \textbf{6.32} & 8.77 & \textbf{6.29} & 8.85 & \textbf{6.19} & 8.89 & \textbf{6.22} & 9.12 \\
    \methodname & \underline{6.45} & \textbf{8.39} & \underline{6.53} & \textbf{8.65} & \underline{6.51} & \textbf{8.71} & \underline{6.43} & \textbf{8.76} & 6.47 & \textbf{9.01} \\
    \bottomrule

  \end{tabular}

% \end{table*}

% \end{subtable}

\bigskip

% \FloatBarrier % This ensures tables stay in place
% \begin{subtable}{0.9\textwidth}
% \begin{table*}[t]
  \centering
  \begin{tabular}{l cc cc cc cc}
    \toprule
    \multirow{2}{*}{Method} & \multicolumn{2}{c}{Lego} & \multicolumn{2}{c}{Stand Up} & \multicolumn{2}{c}{Hellwarrior} & \multicolumn{2}{c}{T-Rex} \\
    \cmidrule(lr){2-3} \cmidrule(lr){4-5} \cmidrule(lr){6-7} \cmidrule(lr){8-9}
    & RGB$\downarrow$ & Depth$\downarrow$ & RGB$\downarrow$ & Depth$\downarrow$ & RGB$\downarrow$ & Depth$\downarrow$ & RGB$\downarrow$ & Depth$\downarrow$ \\
    \midrule
    ARF*~\cite{arf} & \textbf{8.44} & 10.17 & \textbf{8.97} & 10.24 & 8.43 & 9.93 & \textbf{8.83} & 10.26 \\
    Ref-NPR*~\cite{zhang2023ref} & 8.54 & 10.17 & 9.00 & 10.24 & 8.43 & 9.93 & \underline{8.83} & 10.26 \\
    S-DyRF~\cite{li2024sdyrf} & 8.68 & 10.17 & 9.00 & 10.24 & \underline{8.42} & 9.93 & 9.02 & 10.26 \\
    Ours & \underline{8.48} & \textbf{10.06} & \underline{9.00} & \textbf{10.21} & \textbf{8.40} & \textbf{9.90} & 8.85 & \textbf{10.17} \\
    \bottomrule
    % \caption{Quantitative comparisons LPIPS scores for the D-NeRF~\cite{pumarola2020dnerf} dataset with a scene-wise breakdown. The values are scaled by 10 for an increased readability.}
  \end{tabular}

% \end{subtable}

% \end{table}

\captionof{figure}{Quantitative comparisons of LPIPS scores for the NV3D and D-NeRF Dataset, with a scene-wise breakdown of our method, \methodname against the baselines. The values are scaled by a factor of 10 for increased readability.}
\label{tab:lpips_breakdown}
\end{minipage}

\section{Additional Quantitative Results}

We provide an in-depth breakdown of the results presented in ~\Cref{tab:lpips_avg} in ~\Cref{tab:lpips_breakdown}. The results further confirm that our method is able to consistently achieve state-of-the-art performance 

\section{Additional Qualitative Results}
In the accompanying supplementary zip file, we provide numerous video comparisons of our proposed method, \methodname, against the mentioned baselines. The naming convention of the videos is as follows:

"ours\_BASELINE\_SCENE\_STYLE.mp4" 
We also provide the Style images used in these videos in the subfolder called "styles". 

Additionally, we also provide qualitative results with varying time and camera view in ~\Cref{fig:suppl_nv3d_1,fig:suppl_qualitativ_dnerf,fig:suppl_qualitative_nv3d}.

\section{Effect of Joint-Optimization of Geometry and Appearance}
We analyze the impact of simultaneously modifying both geometry and appearance compared to our proposed two-step process in ~\Cref{fig:suppl_stages}. It is evident that with joint optimization, the geometry retains fewer details and remains closer to the original unstylized form.

\begin{figure*}
\begin{minipage}[ht]{0.9\textwidth}
% \raggedleft
% \captionsetup{type=figure,width=.9\textwidth}
\includegraphics[width=\textwidth]{ICCV2025-Author-Kit-Feb/figures/suppl_stages.png}
    \captionof{figure}{We study the effect of jointly modifying the geometry and appearance (right) instead of our proposed 2 step process (left). It can be noticed that when we do joint-optimization, the geometry is still lacking many details and appears more close to the unstylized geometry.}
\label{fig:suppl_stages}
\end{minipage}
\end{figure*}

\begin{figure}[h]
\centering
        \captionsetup{type=figure}
    \includegraphics[width=0.7\textwidth]{ICCV2025-Author-Kit-Feb/figures/suppl_qualitativ_dnerf.png}
    \caption{We provide additional qualitative results on D-NeRF.}
    \label{fig:suppl_qualitativ_dnerf}
\end{figure}

\begin{figure*}[h]
\centering
        \captionsetup{type=figure}
    \includegraphics[width=0.91\textwidth]{ICCV2025-Author-Kit-Feb/figures/suppl_qualitative_nv3d.png}
    \caption{We provide additional qualitative results on the Nv3D dataset.}
    \label{fig:suppl_qualitative_nv3d}
\end{figure*}

\begin{figure*}[h]
\centering
        \captionsetup{type=figure}
    \includegraphics[width=0.9\textwidth]{ICCV2025-Author-Kit-Feb/figures/suppl_nv3d_1.png}
    \caption{We provide additional qualitative results on the Nv3D dataset, interpolating through space-time.}
    \label{fig:suppl_nv3d_1}
\end{figure*}

% \begin{figure*}[h]
% \centering
%         \captionsetup{type=figure}
%     \includegraphics[width=0.9\textwidth]{ICCV2025-Author-Kit-Feb/figures/suppl_nv3d_2.png}
%     \caption{}
%     \label{fig:suppl_nv3d_2}
% \end{figure*}
