# Supplementary material for: GAS-NeRF: Geometry-Aware Stylization of Dynamic Radiance Fields
Source: arXiv:2503.08483 source file (2025-03-11)
Supplement: Supplementary file 2 [file tables_suppl.tex]

% \FloatBarrier % This ensures tables stay in place
% \begin{table}[ht!]

% \begin{subtable}[t]{0.9\textwidth}
  \centering
  \begin{tabular}{l cc cc cc cc cc}
    \toprule
    \multirow{2}{*}{Method} & \multicolumn{2}{c}{Flame Salmon} & \multicolumn{2}{c}{Coffee Martini} & \multicolumn{2}{c}{Cook Spinach} & \multicolumn{2}{c}{Flame Steak} & \multicolumn{2}{c}{Cut Roasted Beef} \\
    \cmidrule(lr){2-3} \cmidrule(lr){4-5} \cmidrule(lr){6-7} \cmidrule(lr){8-9} \cmidrule(lr){10-11}
    & RGB$\downarrow$ & Depth$\downarrow$ & RGB$\downarrow$ & Depth$\downarrow$ & RGB$\downarrow$ & Depth$\downarrow$ & RGB$\downarrow$ & Depth$\downarrow$ & RGB$\downarrow$ & Depth$\downarrow$ \\
    \midrule
    ARF*~\cite{arf} & 6.49 & 8.42 & 6.56 & 8.77 & 6.57 & 8.85 & 6.45 & 8.89 & \underline{6.37} & 9.12 \\
    Ref-NPR*~\cite{zhang2023ref} & 6.56 & 8.42 & 6.70 & 8.77 & 6.69 & 8.85 & 6.69 & 8.89 & 6.77 & 9.12 \\
    S-DyRF~\cite{li2024sdyrf} & \textbf{6.23} & 8.42 & \textbf{6.32} & 8.77 & \textbf{6.29} & 8.85 & \textbf{6.19} & 8.89 & \textbf{6.22} & 9.12 \\
    \methodname & \underline{6.45} & \textbf{8.39} & \underline{6.53} & \textbf{8.65} & \underline{6.51} & \textbf{8.71} & \underline{6.43} & \textbf{8.76} & 6.47 & \textbf{9.01} \\
    \bottomrule

  \end{tabular}

% \end{table*}

% \end{subtable}

\bigskip

% \FloatBarrier % This ensures tables stay in place
% \begin{subtable}{0.9\textwidth}
% \begin{table*}[t]
  \centering
  \begin{tabular}{l cc cc cc cc}
    \toprule
    \multirow{2}{*}{Method} & \multicolumn{2}{c}{Lego} & \multicolumn{2}{c}{Stand Up} & \multicolumn{2}{c}{Hellwarrior} & \multicolumn{2}{c}{T-Rex} \\
    \cmidrule(lr){2-3} \cmidrule(lr){4-5} \cmidrule(lr){6-7} \cmidrule(lr){8-9}
    & RGB$\downarrow$ & Depth$\downarrow$ & RGB$\downarrow$ & Depth$\downarrow$ & RGB$\downarrow$ & Depth$\downarrow$ & RGB$\downarrow$ & Depth$\downarrow$ \\
    \midrule
    ARF*~\cite{arf} & \textbf{8.44} & 10.17 & \textbf{8.97} & 10.24 & 8.43 & 9.93 & \textbf{8.83} & 10.26 \\
    Ref-NPR*~\cite{zhang2023ref} & 8.54 & 10.17 & 9.00 & 10.24 & 8.43 & 9.93 & \underline{8.83} & 10.26 \\
    S-DyRF~\cite{li2024sdyrf} & 8.68 & 10.17 & 9.00 & 10.24 & \underline{8.42} & 9.93 & 9.02 & 10.26 \\
    Ours & \underline{8.48} & \textbf{10.06} & \underline{9.00} & \textbf{10.21} & \textbf{8.40} & \textbf{9.90} & 8.85 & \textbf{10.17} \\
    \bottomrule
    % \caption{Quantitative comparisons LPIPS scores for the D-NeRF~\cite{pumarola2020dnerf} dataset with a scene-wise breakdown. The values are scaled by 10 for an increased readability.}
  \end{tabular}

% \end{subtable}

% \end{table}
